# Supplementary material for: CMM-Math: A Chinese Multimodal Math Dataset To Evaluate and Enhance the Mathematics Reasoning of Large Multimodal Models
Source: arXiv:2409.02834 source file (2024-11-01)
Supplement: Supplementary file 1 [file 07-Appendix.tex]

\clearpage
\section*{Appendix}
\appendix

% \tableofcontents
